# Supplementary material for: DiffusionLight-Turbo: Accelerated Light Probes for Free via Single-Pass Chrome Ball Inpainting
Source: arXiv:2507.01305 source file (2026-01-30)
Supplement: Supplementary file 1 [file additional_object_insertion_halfpage.tex]

% ==============================
% Additional Result for object insertion
% ===============================

\tabulinesep=0.5pt
\begin{figure*}[!t]
    \centering

    \begin{tabu} to \textwidth {
        @{}
        % 1st example
        c@{\hspace{2pt}}
        c@{\hspace{2pt}}
    }

        \multicolumn{1}{c}{\shortstack{ Input object}}
        &
        \multicolumn{1}{c}{\shortstack{Input object}} \\
        \noindent\parbox[c]{0.5\textwidth}{\centering\includegraphics[height=0.2\textwidth]{storage/appendix_object_insertion/input_bag.pdf}} &
        \noindent\parbox[c]{0.5\textwidth}{\centering\includegraphics[height=0.2\textwidth]{storage/appendix_object_insertion/input_shoe.pdf}}
    \end{tabu}

    \begin{tabu} to \textwidth {
        @{}
        % 1st example
        c@{\hspace{2pt}}
        c@{\hspace{2pt}}
        c@{\hspace{2pt}}
        c@{\hspace{2pt}}
    }

        \multicolumn{1}{c}{\shortstack{ Before relighting}}
        &
        \multicolumn{1}{c}{\shortstack{ After relighting}}
        &
        \multicolumn{1}{c}{\shortstack{ Before relighting}}
        &
        \multicolumn{1}{c}{\shortstack{ After relighting}}
        \\ 
        \noindent\parbox[c]{0.23\textwidth}{\includegraphics[height=0.23\textwidth]{storage/appendix_object_insertion_perspective/bedzoom_bag_no_light.pdf}} &
        \noindent\parbox[c]{0.23\textwidth}{\includegraphics[height=0.23\textwidth]{storage/appendix_object_insertion_perspective/bedzoom_bag.pdf}}&
        \noindent\parbox[c]{0.23\textwidth}{\includegraphics[height=0.23\textwidth]{storage/appendix_object_insertion_perspective/bedzoom_shoe_no_light.pdf}} &
        \noindent\parbox[c]{0.23\textwidth}{\includegraphics[height=0.23\textwidth]{storage/appendix_object_insertion_perspective/bedzoom_shoe.pdf}}
        % bag
        \\
        \noindent\parbox[c]{0.23\textwidth}{\includegraphics[height=0.23\textwidth]{storage/appendix_object_insertion_perspective/cambodia2tilt_bag_nolight.pdf}} &
        \noindent\parbox[c]{0.23\textwidth}{\includegraphics[height=0.23\textwidth]{storage/appendix_object_insertion_perspective/cambodia2tilt_bag.pdf}} &
        \noindent\parbox[c]{0.23\textwidth}{\includegraphics[height=0.23\textwidth]{storage/appendix_object_insertion_perspective/cambodia2tilt_shoe_nolight.pdf}} &
        \noindent\parbox[c]{0.23\textwidth}{\includegraphics[height=0.23\textwidth]{storage/appendix_object_insertion_perspective/cambodia2tilt_shoe.pdf}}
    \end{tabu}
    \caption{
    We synthetically render each 3D object into input images using our estimated lighting.
    %results for virtual object insertion.
    }
    \label{fig:additional_object_insertion}
\end{figure*}
